# Supplementary material for: Post-hoc Bias Scoring Is Optimal For Fair Classification
Source: arXiv:2310.05725 source file (2024-03-15)
Supplement: Supplementary file 1 [file multi.tex]

Suppose, we have a multi-class classification problem $Y = 1, \dots, k$. Suppose we have $p(Y = y, A = a| X)$ for each $y = 1, \dots, k$, $a = 0, 1$. We want to equalize,
\[
    DP(\hat{Y}) = \max_{y = 1, \dots, k} \left| \Pr(\hat{Y} = y | A = 0) - \Pr(\hat{Y} = y | A = 0) \right|
\]

Bayes optimal classifier,
\[
    \hat{Y}(X) = \arg\max_{j = 1, \dots, k} p(Y = j | X) 
\]

Set, $ f_{j}(X) = p(Y = j, A = 0) / \Pr(A = 0) - p(Y = j, A = 1) / \Pr(A = 1) $. Then, we will show (to be confirmed), that optimal classifier under DP restriction has the form
\[
    \hat{Y}(X) = \arg\max_{j = 1, \dots, k} \left[ p(Y = j | X) + z_{j} f_{j}(X) \right],
\]
with the number of parameters $z_1, \dots, z_{k}$ now being proportional to the class number. Potentially, there can be more group restrictions, so that we replace with a sum $\sum_{l} z_{jl} f_{jl}(X)$.

Another problem is to consider equalized accuracy
\[
    C(\hat{Y}) = \max_{y = 1, \dots, k} \left| \Pr(\hat{Y} = y | Y = y) - Acc(\hat{Y}) \right|
\]

Check BER/

\[
    C(\hat{Y}) = \max_{g = 1, \dots, k} \left| \Pr(\hat{Y} = Y | g) - Acc(\hat{Y}) \right|
\]
